# Supplementary material for: On the bias of K-fold cross validation with stable learners
Source: arXiv:2202.10211 source file (2023-06-11)
Supplement: Supplementary file 1 [file appendix.tex]

First we derive a probability upper bound for $\DevCV$ defined in \ref{def:dev_CV}.

\begin{lemma}\label{lemma:Dev-CV-UB}
 Suppose that Assumption~\ref{assum:stability-setting} holds with $\beta_n=\ffrac{\lambda}{n}$, for some $\lambda>0$. Then, for all CV schemes verifying Assumption \ref{assum:mask-property},  we have, with probability $1-\delta$,
	\begin{equation*}
	\PP(\abs{\DevCV} \geq t) \leq 2\exp{\left(\ffrac{-nt^2}{16(\lambda+L)^2} \right)}.
	\end{equation*}
	Where $L$ is the upper bound of the cost function.
\end{lemma}
\begin{proof} 
	The proof of this lemma relies on Mcdiarmid's inequality. 
	
	Let  $O'\in \mathcal{X}$ be  an independent copy of $O_1,O_2,\dots,O_n$,\,for some $l\in \llbracket1,n\rrbracket$ define 
	
	\[\Delta_l(\DD,O')=\big\lvert \DevCV(\DD)-\DevCV(\DD^l)\big\rvert, \]
	
	where $\DD^{l}$ is obtained by replacing the $l$'th element of $\DD$ by $O'$. Furthermore write $\DevCV$ under the following form,
	\begin{align*}
	\DevCV&=\rCV(\alg,V_{1:K})-  \risk_{CV}(\alg,V_{1:K})\\
&=\frac{1}{Kn_{val}}\sum_{j=1}^K\sum_{i \in V_j} \bigg(\loss(\algdd (T_j),O_i)-\EE\big[\loss(\algdd(T_j),O_i) \mid \DD_{T_j})\big]\bigg)\\
	&=\frac{1}{Kn_{val}}\sum_{j=1}^K\sum_{i \in V_j}h_{i,j}(\DD)
	\end{align*}
	
	Notice that for a training mask $T_j\subset [n]$, the training set $\DD_{T_j}^{l}=\{O_i \in \DD^{l,O'} \mid i \in T_j\}$ verifies for all $ \DD_{T_j},o \in \mathcal{Z}^{n_{T}}\times \mathcal{Z}$,
	\begin{equation}
	\label{"train_set_dev"}
	\begin{cases}
	\loss\big(\algdd(T_j),o\big)=\loss\big(\algcg(T_j),o\big)\: \text{if} \: l \notin T_j\\
	\bigg \lvert \loss\big(\algdd(T_j),o\big)-\loss\big(\algcg(T_j),o\big) \bigg\rvert \leq 2\beta_{n_{T}}\:,\: \text{otherwise}.
	\end{cases}
	\end{equation}
	The first equation follows from the fact that $\DD_{T_j}^{l}=\DD_{T_j}$ if $l\notin T_j$,\,indeed,\,if the training set $\DD_{T_j}$ doesn't contain the index $l$ then changing the $l$'th element of $\DD$ won't affect $\DD_{T_j}$.\,The second inequality is obtained using the \emph{leave-one-out} stability of $\alg$ and corollary \ref{lemma:uniform-stab-link}.\\ 
	On the other hand write, for $O_i \in \DD_{V_j}$  
	
	\begin{equation*}
	\eqref{"train_set_dev"} \implies
	\begin{cases}
	\EE_{O_i}\bigg[\loss\big(\algdd(T_j),O_i\big)\bigg]=\EE_{O_i}\bigg[\loss\big(\algcg(T_j),O_i\big)\bigg]\: \text{if} \: l \notin T_j\\
	\bigg \lvert \EE_{O_i}\big[\loss\big(\algdd(T_j),O_i\big)-\loss\big(\algcg(T_j),O_i\big) \big]\bigg\rvert \leq 2\beta_{n_{T}} , \: \text{otherwise}.
	\end{cases}
	\end{equation*}
	Where $\EE_{O_i}$ is the expectation with respect to $O_i$. Since the above equation holds $\forall \DD_{T_j},O'$  and since $O_i\in \DD_{V_j}$ is independent from $\DD_{T_j}$,\,conclude
	\begin{equation}
	\label{"expectation_train_set_dev"}
	\begin{cases}
	\EE\bigg[\loss\big(\algdd(T_j),O_i\big)\mid \DD_{T_j}\bigg]=\EE\bigg[\loss\big(\algcg(T_j),O_i\big)\mid \DD_{T_j}^{l}\bigg]\: \text{if} \: l \notin T_j\\
	\bigg \lvert \EE\big[\loss\big(\algdd(T_j),O_i\big)\mid\DD_{T_j}\big] -\EE\big[\loss\big(\algcg(T_j),O_i\big)\mid  \DD_{T_j}^{l} \big]\bigg\rvert \leq 2\beta_{n_{T}} , \: \text{otherwise}.
	\end{cases}
	\end{equation}
	Combining \eqref{"expectation_train_set_dev"} and \eqref{"train_set_dev"} gives
	\begin{equation*}
	\abs{\un{l \in T_j}(h_{i,j}(\DD)-h_{i,j}(\DD^l))} \leq 4\beta_{n_{T}}
	\end{equation*}
	\begin{equation*}
	\abs{\underbrace{\un{l \notin T_j}}_{\un{l \in V_j}}(h_{i,j}(\DD)-h_{i,j}(\DD^{l})) }\leq 4C\un{i=l}.
	\end{equation*}
	Finally obtain 
	\begin{align*}
	\abs{\Delta_l(\DD,O')}&\leq \ffrac{4\beta_{n_{T}}}{K}\sum_{j=1}^{K}\un{l \in T_j} +\ffrac{4C}{n_{val}K}\sum_{j=1}^{K}\un{l \in V_j}\\
	(\text{by assumption \ref{assum:mask-property}} )   &\leq \ffrac{4\beta_{n_{T}} n_{T}}{n}+\ffrac{4C}{n}.
	\end{align*}
	Using Mcdiarmid's inequality ( proposition \ref{prop:Mcdiarmids-ineq}) gives,
	\begin{equation*}
	\PP(\DevCV \geq t) \leq \exp{\left(\ffrac{-nt^2}{16(\beta_{n_{T}}n_{T}+C)^2} \right)}.
	\end{equation*}
	Symmetrically, one has,
	\begin{equation*}
		\PP(\DevCV \leq -t) \leq \exp{\left(\ffrac{-nt^2}{16(\beta_{n_{T}}n_{T}+C)^2} \right)}.
	\end{equation*}
	Thus,
	$$ \PP(\abs{\DevCV} \geq t) \leq 2\exp{\left(\ffrac{-nt^2}{16(\beta_{n_{T}}n_{T}+C)^2} \right)}. $$
	Reminding that $\beta_n=\lambda/n$  yields the desired result. 
\end{proof}
Using the same steps as previously we can show that a similar inequality holds for $\DevT$,
\begin{lemma}\label{lemma:Dev-train-UB}
	Suppose that Assumption~\ref{assum:stability-setting} holds with $\beta_n=\ffrac{\lambda}{n}$, for some $\lambda>0$. Then, for all CV schemes verifying Assumption \ref{assum:mask-property},  we have,
	\begin{equation*}
		\PP(\abs{\DevT-\frac{2\lambda}{n_T}} \geq t) \leq 2\exp{\left(\ffrac{-nt^2}{16(\lambda+L)^2} \right)}.
	\end{equation*}
	Where $\DevT$ is defined in \ref{def:dev_train} and $L$ is the upper bound of the cost function. 
\end{lemma}
	\begin{proof}
		 As previously, the idea consists on using Mcdiarmid's inequality. Similar argument can be used to bound the term $\Delta$ corresponding to the maximum deviation of  $\DevT$. In fact, for $\DD,O' \in \mathcal{Z}^n\times \mathcal{Z}$, one has,
		 \[\Delta_l(\DD,O')=\big\lvert \DevT(\DD)-\DevT(\DD^l)\big\rvert \leq \ffrac{4\beta_{n_{T}} n_{T}}{n}+\ffrac{4C}{n}. \]

		 However, this time $Z=\DevT$ is not centered. To control $\EE[Z]$, notice that
		
		$$\EE(Z) =\EE\left[\risk\left[\algdd(T_1)\right]-\ER\left[\algdd(T_1),T_1\right]\right] $$
		Then, borrow lemma 7 from \cite{bousquet2002stability}  that says that,
		\begin{equation}\label{ineq:stability-expectation-UB}
		\forall T\subset [n] \quad , \quad	\EE\left[\risk\left[\alg(T)\right]-\ER\left[\alg(T),T\right]\right]= \EE\left[\loss\left(\alg(\DD_{T}),O'\right)-\loss\left(\alg(\DD_{T}^{l}),O'\right)\right].
		\end{equation}
		Where  $\DD_T^{l}$ is obtained by replacing the $l$'th element of $\DD_T$ by $O'$.
		Replacing the left side term by $\EE[Z]$ and using corollary \ref{lemma:uniform-stab-link} gives,
		\begin{equation}
		\abs{\EE[Z]} \leq 2\beta_{n_{T}}
		\end{equation}
		Thus by Mcdiarmid's, we obtain,
		\begin{equation*}
			\PP(Z-\frac{2\lambda}{n_T} \geq t) \leq \exp{\left(\ffrac{-nt^2}{16(\lambda+L)^2} \right)}.
		\end{equation*}
		Symmetrically, one has,
				\begin{equation*}
			\PP(-Z+\frac{2\lambda}{n_T} \leq -t) \leq \exp{\left(\ffrac{-nt^2}{16(\lambda+L)^2} \right)}.
		\end{equation*}
	Thus,
		\begin{equation*}
		\PP(\abs{Z-\frac{2\lambda}{n_T}} \geq t) \leq 2\exp{\left(\ffrac{-nt^2}{16(\lambda+L)^2} \right)}.
	\end{equation*}
		It remain to use the fact that $\beta_n=\ffrac{\lambda}{n}$ and the proof is complete .
	\end{proof}
\begin{proposition}\label{prop:uniform-CVC-UB}
	Let $(\alg^{(m)})_{m\in \mathcal{M}}$ be a family of algorithms where each learner $\alg^{(m)}$ is $(\ffrac{\lambda_m}{i})_{1\leq i \leq n}$ uniform stable with respect to loss function $0\leq \loss(g,O)\leq L$. Additionally, assume that, $\abs{\mathcal{M}}< \infty$ and,
	$$ \forall m \in \mathcal{M} \:;\: \lambda_m \leq M,$$
	for some $M>0$. Then one has, with probability at least $1-6\delta$,
	\begin{align*}
	\sup_{m\in \mathcal{M}}\bigg|\rCVC(\alg^{(m)},V_{1:K})-\TR\big[&\algdd^{(m)}([n])\big]\bigg|\leq  4M(\ffrac{1}{n}+\ffrac{1}{n_T})\\ &+8(M+L)\sqrt{\ffrac{\log(\mathcal{\abs{M}})\log(1/\delta)}{n}}.
	\end{align*}
\end{proposition}
\subsection{Proof of Lemma \ref{lemma:uniform-stab-link}}
It suffices to notices that,
	\begin{align*}
	\abs{\loss\big(\algdd(T),O\big)-\loss\big(\algdd(T^i,O\big)} &\leq \abs{\loss\big(\algdd(T),O\big)-\loss\big(\algdd(T^{\backslash i}),O\big)} + \abs{\loss\big(\algdd(T^{\backslash i}),O\big)-\loss\big(\algdd(T^i),O\big)}\\
	&\leq 2\beta_{\abs{T}},
\end{align*}
and the proof is complete.	
\subsection{Proof of Theorem \ref{theo:CV-stable-bound}}\label{proof:CV-UB}
We follow the same steps as in the sketch of proof. Using equation \ref{ineq:error-decomp}, write ,
\begin{align*}
	\rCV(\alg,V_{1:K})-\TR\big[\algdd([n])\big] \leq \abs{\DevCV}+\abs{\BiasCV}.
\end{align*}	
It remains to combine Lemma \ref{lemma:Dev-CV-UB} with Lemma \ref{corro:Bias-UB} and the proof is complete.

\subsection{Proof of Theorem \ref{theo:CVC-UB-det}}\label{proof:CVC-UB}
We proceed as described in sketch of the proof. First remind the error decomposition \ref{ineq:error-decom-cvc},
$$ \rCVC(\alg,V_{1:K})-\risk(\alg[n]) = \DevT + \DevCV + \DevAll $$ 

Where $\DevCV$, $\DevT$ and $\DevAll$ are defined in \ref{def:dev_CV}, \ref{def:dev_train} and \ref{def:dev_all} respectively.

Combining lemma \ref{lemma:Dev-CV-UB} and \ref{lemma:Dev-train-UB} regarding $\DevCV$ and $\DevT$ with proposition \ref{prop:ER-stability-bound} regarding $\DevAll$, one obtains, with probability $1-6\delta$,
$$\rCVC(\alg,V_{1:K})-\risk(\alg[n]) \leq 2\lambda(\ffrac{1}{n}+\ffrac{1}{n_T}) +4(\lambda+C)\sqrt{\ffrac{\log(1/\delta)}{n}} $$.
Which is the desired result.

\subsection{Proof of Theorem \ref{theo:K-fold-LB}}\label{sec:proof-LB}

We follow the steps from sketch of proof. To prove the boundness of $\loss$ on $\mathcal{Z}$ (step 1) it suffices to show that, 
\begin{align*}
	 S_n = \sum_{j= 1}^{n}(1/j) &\leq \log(n)+1\\
	(n \leq \exp(L)) &\leq L^2 +1
\end{align*}

Indeed, write, 
\begin{align*}
\log(n)=\int_{1/n}^{1}\frac{dx}{x}&=
\sum_{j=1}^{n-1}\int_{1/(j+1)}^{1/j}\frac{dx}{x}\\
& \geq	\sum_{j=1}^{n-1}\frac{1}{j+1}\\
&= S_n-1,
\end{align*}
which concludes the first step. Now, let's check that our learning rule defined in \ref{def:alg-LB} is $\lambda/n$ uniform stable. First, notice that under the assumption $0\leq \lambda \leq L(1+\frac{2}{n})^{-1}$ and $0\leq\epsilon\leq \frac{\lambda}{n}$, one has,
$$\alg_{\DD}(T,x_m)\leq x_m,$$
where $x_m=\sigma_m\varepsilon + LS_m$ is an element of $\mathcal{X}$ (cf. eq \ref{def:X-LB}). Thus, for any $O_m=(x_m,x_m)\in \mathcal{Z}$,
\begin{equation}\label{eq:loss-formula}
	\loss(\algdd(T),O_m)=x_m-\algdd(T,x_m).
\end{equation}

Using equation \ref{eq:loss-formula} and the triangular inequality yields,
\begin{align*}
   \abs{\loss(\algdd(T),O)- \loss(\algdd(T^{\backslash j}),O)}&\leq  \lambda\abs{S_{\min(m,n_{T})}-S_{\min(m,n_{T}-1)}}+2\varepsilon\\
   &=\begin{cases}
   	2\varepsilon + \frac{\lambda}{n_{T}} \quad \text{if} \quad i= n_T\\
   	2\varepsilon 	\quad \text{otherwise}
   \end{cases}\\
(\varepsilon\leq \frac{\lambda}{n_T})  &\leq \frac{3\lambda}{n_T}. 
\end{align*} 

Consequently, $\alg$ is $\ffrac{3\lambda}{n}$ leave-one-out stable. Now, let's compute the true risk of our algorithm, since P is the uniform distribution over $\mathcal{Z}$, we can write, for any $T\subset[n]$,

\begin{align*}
	\risk(\algdd(T))&=\EE[\alg_{\DD}(T),O \mid \DD_T]\\
	&=\ffrac{1}{n}\sum_{x_m \in \mathcal{Z}}\loss(\algdd(T),x_m)\\
(\text{By }\ref{eq:loss-formula})	&=\ffrac{1}{n}\sum_{m=1}^{n}(x_m-\algdd(T,x_m))\\
	&=\ffrac{1}{n}\sum_{m=1}^{n}\left(LS_m-\lambda S_{\min(n_T,m)}+ \varepsilon\sign(\med(\DD_T)-x_m)\right)
\end{align*}

Thus, one obtains with simple algebra,
\begin{equation}\label{ineq: bias-LB}
	\ffrac{\lambda}{n}\sum_{m=(n_{T}+1)}^{n}(S_m-S_{n_T})-2\varepsilon  \leq \risk(\algdd(T))- \risk(\algdd([n]))  
\end{equation}

It remains to derive a lower bound for the left side term in the above equation, to do so write,

\begin{align*}
	\ffrac{\lambda}{n}\sum_{m=(n_{T}+1)}^{n}(S_m-S_{n_T})-2\varepsilon &=\ffrac{\lambda}{n}\sum_{m=(n_{T}+1)}^{n}(\sum_{j=(n_{T}+1)}^{m}\frac{1}{j})-2\varepsilon\\
(\frac{1}{j} \geq \frac{1}{n} )	&\geq \ffrac{\lambda}{n^2}\sum_{m=(n_{T}+1)}^{n}(m-n_{T}-1)-2\varepsilon\\
(n_V=n-n_T)&\geq \ffrac{\lambda}{n^2}\sum_{m=1}^{n_V}m-2\varepsilon\\
(\varepsilon \leq \ffrac{\lambda}{n})&\geq \lambda\ffrac{n_V^2}{2n^2} - \ffrac{2\lambda}{n}\\
(n_V=\ffrac{n}{K})&\geq \ffrac{\lambda}{2K^2} - \ffrac{2\lambda}{n}.
\end{align*}

Injecting the above inequality in equation \ref{ineq: bias-LB} gives, 
\begin{equation}\label{ineq:bias-Kfold-LB}
\ffrac{\lambda}{2K^2} - \ffrac{2\lambda}{n}	 \leq \risk(\algdd(T))- \risk(\algdd([n])). 
\end{equation}

On the other hand, an application of the tower rule yields,
\begin{align*}
	\EE\left[\bigg|\rCV(\alg,V_{1:K})-\risk\left[\alg_{\DD}([n])\right]\bigg|\right] &= \EE\left[\bigg|\ffrac{1}{K}(\sum_{j=1}^{K}\risk\left[\alg_{\DD}(T_j)\right]-\risk\left[\alg_{\DD}([n])\right])\bigg|\right]\\
\big( \risk(\algdd(T_j))\geq \risk(\algdd([n]))\big)	&=\EE\left[\ffrac{1}{K}(\sum_{j=1}^{K}\risk\left[\alg_{\DD}(T_j)\right]-\risk\left[\alg_{\DD}([n])\right])\right]
\end{align*}

Which, using \ref{ineq:bias-Kfold-LB}, gives the desired result.
